# Supplementary material for: The time-dependent $CP$ asymmetry in $B^0 \to K_{\rm res} \gamma \to \pi^+ \pi^- K^0_{\scriptscriptstyle S} \gamma$ decays
Source: arXiv:1802.09433 source file (2019-09-09)
Supplement: Supplementary file 1 [file appendix_Babar.tex]

%%%%%%%%%%%%%%%%%%%%%%%%%%%%%%%%%%%%%%%%
\appendix
\section{The parameterisation used by \babar}
\label{App:BabarParam}

Here, we remind the parameterisation used by the \babar collaboration in Ref.~\cite{Sanchez:2015pxu}. \emi{First of all, we introduce the $F_i^{\pm}$ ($i=\rho, \Kst, \swave$) parameters used therein.} 
\begin{eqnarray}
	&& F_{\rho}^{+} \equiv \AmpTot^{\rhoz \Kp}, \, F_\rhoz^-\equiv \AmpTot^{\rho \Km}, \, F_{\Kst}^+\equiv \AmpTot^{K^{*0} \pip}, \nonumber \\
	&& F_{\Kst}^-\equiv \AmpTot^{\overline{K}^{*0}\pim}, \ F_{\swave}^+\equiv \AmpTot^{\swave \pip}, \ F_{\swave}^-\equiv \AmpTot^{(\overline{K}\pi)_0\pim}, 	
\end{eqnarray}
\emi{where the amplitudes on the right hand sides are those used in this paper.} 
As described in the previous sections, we do not expect any direct \CP asymmetry.  Therefore, $B^{+}$ and $B^{-}$ amplitudes are the same up to the sign.\footnote{Strictly speaking, under the assumption of no direct \CP violation, we are left with a sign ambiguity:
\[  F_{\rho} = F_{\rho}^+=F_{\rho}^-, \quad  F_{\Kst} =  e^{i\delta_{\rm rescat.}} F_{\Kstp} = F_{\Kstm}\]
with $\delta_{\rm rescat.} = 0$ or $\pi$. 
For $\delta_{\rm rescat.} = \pi$, the sum of the interference of $F_\rho^+, F_{\Kstp}$ and $F_\rho^-, F_{\Kstm}$ would have been zero while Ref.~\cite{Sanchez:2015pxu} reports a sizable interference. Thus, we keep only $\delta_{\rm rescat.} = 0$. 
Similar expressions can be derived for the $\swave \pip$ terms.}
Thus, we also define $F_i\equiv F^+_i=F^-_i$.
Then, the isospin symmetry can relate the amplitudes of \Bz(\Bzb) decay in \Eqref{seq:v2_28} to these  \Bp(\Bm) amplitudes as 
\begin{equation}
\AmpTotRhoKs=\frac{F_\rho}{\sqrt{2}}, \quad 
\AmpTotKstPi=\frac{F_{\Kst}}{\sqrt{2}}, \quad 
\AmpTotKappaPi=\frac{F_{\swave}}{\sqrt{2}},
\end{equation}
where the factor $1/\sqrt{2}$ comes from $\KS=\frac{K^0+\overline{K}^0}{\sqrt{2}}$. 
Then, the terms in \Eqref{seq:v2_28} can be re-written as:  
\begin{eqnarray}
\sumLR{ \ModSq{\AmpTotRhoKs} } & =&{\ModSq{F_{\rho}}},\\
\sumLR{ \ModSq{\AmpTotKstPi} } & = &{\ModSq{F_{\Kst}}},\\
\sumLR{ \ModSq{\AmpTotKappaPi} } & = &{\ModSq{F_{\swave}}}, \\
\sumLR{ 2\Real{\AmpTotRhoKsConj \AmpTotKstPi} } & = &  2\Real{F^{*}_{\rho} F_{\Kst}},\\
\sumLR{ 2\Real{\AmpTotRhoKsConj \AmpTotKappaPi} } & = & 2\Real{F^{*}_{\rho} F_{\swave}}, \\
\sumLR{ \Real{\AmpTotBarKstPiConj \AmpTotKstPi} } & = &  \Real{F^{*+}_{\Kst} F^{-}_{\Kst}},\label{eq:sv2_36}\\
\sumLR{ \Real{\AmpTotBarKappaPiConj \AmpTotKappaPi} } & = & \Real{F^{*+}_{\swave} F^-_{\swave}}. \label{eq:sv2_37}
\end{eqnarray}
It should be noted that in the analysis of~\cite{Sanchez:2015pxu}, \Bp and \Bm decays are not treated separately. Thus, the right-hand-side of these equations are understood as an average 
$\ModSq{F_i} = \frac{ \ModSq{F_i^+} + \ModSq{F_i^-}}{2}$ and $\Real{F_i^{*} F_j}=\frac{\Real{F_i^{+*}F_j^+}+\Real{F_i^{-*}F_j^-}}{2}$. We should re-emphasize (c.f. see \Eqref{eq:sv2_25}) that the expressions in \Eqsref{eq:sv2_36}{eq:sv2_37} are symbolic since \Bp and \Bm decays do not interfere (unlike \Bz and \Bzb decays, which do interfere). 
In practice, we have to re-caluculate the interference after extracting $F_{\Kst}$: we compute the interference of $F_{\Kstp}$ and  $F_{\Kstm}$ with $p_1$ and $p_2$ exchanged (and similar for \swave).
